# Supplementary material for: Morphology of Fly Larval Class IV Dendrites Accords with a Random Branching and Contact Based Branch Deletion Model
Source: arXiv:1611.05918 ancillary file (2016-11-17)
Supplement: Supplementary file 1 [file GangulyNeuronGrowthSupplement.pdf]

# Morphology of Fly Larval Class IV Dendrites Accords with a Random Branching and Contact Based Branch Deletion Model - Supplementary Information

Sujoy Ganguly, Olivier Trottier, Xin Liang, Hugo Bowne-Anderson, Jonathon Howard
(Dated: November 17, 2016)

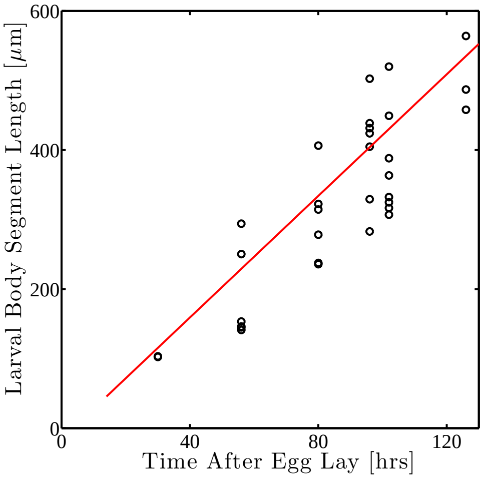


FIG. 1: **Larval Body Segment Length versus Time:** In black are the larval body segment lengths of 32 larvae plotted versus their developmental age. In red is a linear fit to the data. The fit is forced to have a body segment length of 50 $\mu$m at 14 hours after egg lay. The slope of the fit is 4.37 $\mu$m hour$^{-1}$.

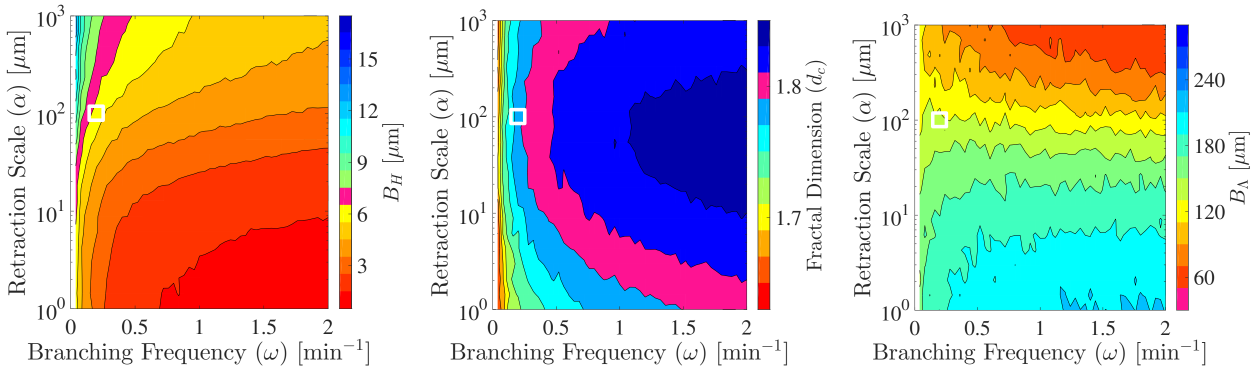


(a)$B_h$ for $\beta = 35\,\mu$m (b)$d_{\rm f}$ for $\beta = 35\,\mu$m (c)$B_\Lambda$ for $\beta = 35\,\mu$m

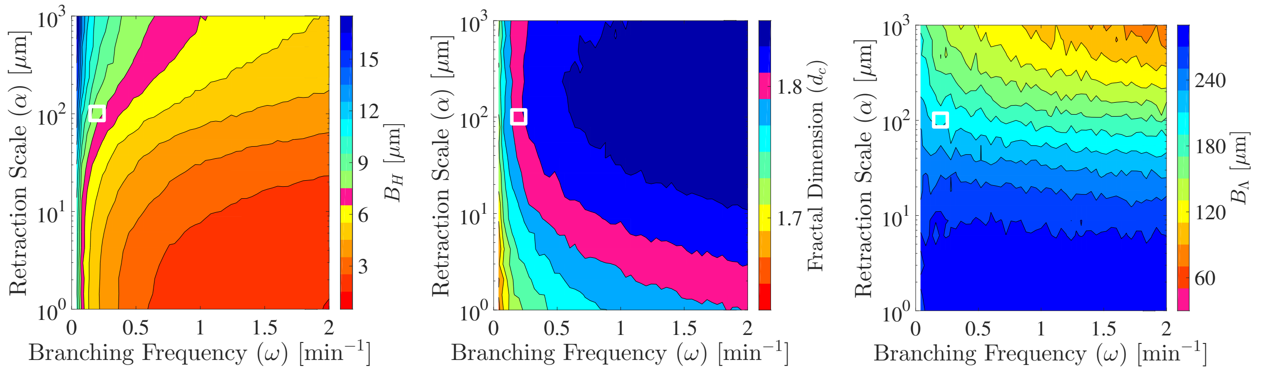


(d)$B_h$ for $\beta = 280\,\mu$m (e)$d_{\rm f}$ for $\beta = 280\,\mu$m (f)$B_\Lambda$ for $\beta = 280\,\mu$m

FIG. 2: **Figure Title** In figures (a), (b) and (c), we have plotted the mesh size $B_h$, fractal dimension $d_{\rm f}$ and lacunarity scale $B_\Lambda$ respectively, versus retraction scale $\alpha$ and branching frequency $\omega$ for $\beta = \{35, 280\}\,\mu$m. The white boxes indicate the parameter set used for the time series comparison ($\omega = 0.2\,{\rm min}^{-1}$ and $\alpha = 100\,\mu$m). As we can see, changing the persistence length does not affect the structure of the contour maps, but simply translates them. This implies that the curvature of the contours are independent of the persistence length, up to an additive or multiplicative factor.

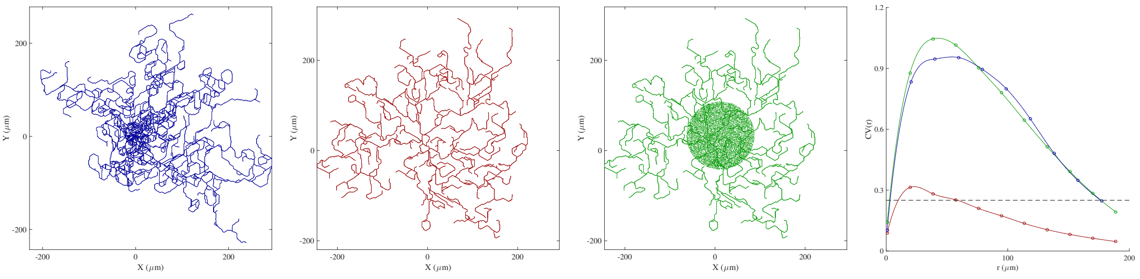

(a)Low $\alpha$ Neuron (b)High $\alpha$ Neuron (c)High $\alpha$ Neuron with an artificial core (d)Lacunarity Curves

FIG. 3: **Effect of high-density cores on $CV(R)$.** In this figure, we analyze the effect of highly-densed regions surrounding the soma on the coefficient of variation $CV(R)$. First, we generated a neuron (a) with $\alpha = 0.4\,\mu$m$, \beta = 100\,\mu$m$, \omega = 0.2$min$^{-1}$, which is considered a low $\alpha$ neuron. Then, we generated a second neuron (b) with $\alpha = 400\,\mu$m$, \beta = 100\,\mu$m$, \omega = 0.2$min$^{-1}$, which has a high $\alpha$. Finally, we took the high $\alpha$ neuron and increased the density of branches close to the soma creating a third neuron (c). Our goal was to mimic the presence of a high-density region similar to neuron (a). This region was defined as a disk centered at the center of mass with a radius $r = R_{\rm g}/2$. To increase the density, we randomly occupied $\frac{1}{10}$ of the lattice points contained in it. Then, we compared the $CV(R)$ curves of all three neurons. As we expected, the low $\alpha$ neuron and the high $\alpha$ alpha with an artificial dense core have very similar $CV(R)$ curves with $B_\Lambda = 176\,\mu$m for both neurons.
